# Supplementary material for: A Constant Factor Approximation for Navigating Through Connected Obstacles in the Plane
Source: arXiv:2011.14463 source file (2020-11-29)
Supplement: Supplementary file 1 [file appendix.tex]

\section{Small-Diamater Decomposition of Region Intersection Graphs}
\label{sec:rig-separators}
	We will need to revisit some basic definitions from~\cite{lee2016separators}.
	We say that a graph $G = (V, E)$ is a \emph{region intersection} graph 
	over the \emph{base} graph $G_0 = (V_0, E_0)$ if for every $u \in V$ there
	exists a connected set of vertices $R_u \subseteq V_0$ such that
	$(u, v) \in E$ if and only if $R_u \cap R_v \neq \emptyset$.

	Now suppose $G$ is vertex-weighted graph with $w(v) > 0$,
	we can define a length value of $\left(w(u) + w(v)\right)/2$ 
	on each edge $(u, v) \in E$ and let $d_w$ be the induced shortest path metric.
	The diameter of a vertex set $X \subseteq V$ is $\sup_{u, v \in X} d(u, v)$.

	For any \emph{center} vertex $c \in V$, define a ball centered at $c$ of radius $R \geq 0$ as
	\begin{align*}
		\cb(c, R) = \left\{ v \in V : d(c, v) < R - \frac{w(v)}{2} \right\}
	\end{align*}

\begin{definition}
A distribution over subsets $S \subseteq V$ is an \emph{$(\alpha, \Delta)$-random separator} if :
\begin{enumerate}
	\item For all $v \in V$ and $R \geq 0$, probability $\mathbf{P}[~\cb(v, R)$ does not intersect $S~] ~\geq~ 1 - \alpha \frac{R}{\Delta}$,
	\item The diameter of every component of $G - S$ (in the metric $d$) is at most $\Delta$
\end{enumerate}
\end{definition}

We now state the main result of Lee~\cite{lee2016separators} relevent to us.
\begin{theorem}[Corollary 4.3 in~\cite{lee2016separators}~]
	\label{thm:rig-separators}
	If $G$ is a region intersection graph over $G_0$ such that $G_0$ excludes $K_h$ as a
	minor, then $G$ admits an $(\alpha, \Delta)$-random separator with $\alpha = O(h^2)$. 
\end{theorem}

With these definitions in place, we can easily obtain the following lemma.
\begin{lemma}
	Let $w(X) = \sum_{v\in X} w(v)$ denote the weight of vertex set $X$.
	Let $S$ be an $(\alpha, \Delta)$-random separator of $G$, then each component 
	has diameter is at most $\Delta$ and the weight $w(S) = O(\frac{\alpha}{\Delta}) \cdot w(V)$
\end{lemma}

\begin{proof}
	Since $S$ is an $(\alpha, \Delta)$-random separator, we have that $\mathbf{P}[~\cb(v, R)$ intersects $S~] \leq \alpha \frac{R}{\Delta}$.
	Now suppose we set $R = w(v)$, then the ball $\cb(v, R)$ only contains the vertex $v$.
	Therefore, $\mathbf{P}[~\cb(v, R)$ intersects $S~] = \mathbb{P}[v \in S~] ~\leq~ \alpha \frac{w(v)}{\Delta}$, and 
	hence the expected weight of the separator $S$ is $O(\frac{\alpha}{\Delta}) \cdot w(V)$.
\end{proof}

The construction of $(\alpha, \Delta)$-random separator in~\cite{lee2016separators} is based on the
well-known iterative chopping scheme of Klein, Plotkin and Rao~\cite{klein1993excluded} and can be
translated into a deterministic algorithm that runs in polynomial time by trying all possible chop values.
